# Supplementary material for: Matching Models for Graph Retrieval
Source: arXiv:2110.00925 source file (2022-04-21)
Supplement: Supplementary file 1 [file appendix.tex]

\appendix
\chapter{First Appendix}
